# Supplementary material for: Cross-Attention Head Position Patterns Can Align with Human Visual Concepts in Text-to-Image Generative Models
Source: arXiv:2412.02237 source file (2025-02-24)
Supplement: Supplementary file 1 [file Appendix_image_editing_ablating_concept_strengthening.tex]

\begin{table}[h]
\caption{Ablation on concept strengthening in Amplified-P2P - CLIP image-text similarity}
\centering
\resizebox{\linewidth}{!}{%
\begin{tabular}{l|c|c|c||c|c}
\hline
\multirow{2}{*}{\textbf{Method}} & \multicolumn{3}{c||}{\textbf{Object Attribute}}                                                                                   & \multicolumn{2}{c}{\textbf{Image Attribute}} \\ \cline{2-6}
                                 & \multicolumn{1}{c|}{\textbf{Color}} & \multicolumn{1}{c|}{\textbf{Material}} & \multicolumn{1}{c||}{\textbf{Geometric Patterns}}  & \multicolumn{1}{c|}{\textbf{Image Style}} & \multicolumn{1}{c}{\textbf{Weather Conditions}} \\ \hline
P2P                                      & 0.3076          & 0.3079          & 0.2593          & 0.3120            & 0.2788    \\
P2P-HRV w/o concept strengthening  & 0.3146          & 0.3125          & 0.2819          & 0.3103            & 0.2849    \\
P2P-HRV (Ours)                     & \textbf{0.3301} & \textbf{0.3466} & \textbf{0.3081} & \textbf{0.3424}   & \textbf{0.3348} \\ 
\hline
\end{tabular}%
}
\label{tab:appendix_image_editing_ablating_concept_strengthening}
\end{table}
