# Supplementary material for: Cross-Attention Head Position Patterns Can Align with Human Visual Concepts in Text-to-Image Generative Models
Source: arXiv:2412.02237 source file (2025-02-24)
Supplement: Supplementary file 2 [file Appendix_misinterpretation_failure_prompt_list.tex]

\begin{table}[h]
\caption{Prompt list for resolving misinterpretation of polysemous words; failure cases}
\centering
\resizebox{0.8\linewidth}{!}{%
\begin{tabular}{l|l|l}
\specialrule{1.1pt}{0pt}{0pt}
\textbf{Prompt}                    & \textbf{Desired Concept} & \textbf{Undesired Concept}    \\ \hline
A single rusted {\ul nut}                & Tools            & Food and Beverages \\
A single rusted {\ul nut}                & Tools            & Food and Beverages \\
A single rusted {\ul nut}                & Tools            & Food and Beverages   \\ \specialrule{1.1pt}{0pt}{0pt}
\end{tabular}}
\label{tab:appendix_misinterpretation_failure_prompt_list}
\end{table}
