# Supplementary material for: Cross-Attention Head Position Patterns Can Align with Human Visual Concepts in Text-to-Image Generative Models
Source: arXiv:2412.02237 source file (2025-02-24)
Supplement: Supplementary file 3 [file Appendix_misinterpretation_human_evaluation.tex]

\begin{table}[h]
\caption{Human evaluation results on resolving misinterpretation of polysemous words}
\centering
\resizebox{0.8\linewidth}{!}{%
\begin{tabular}{l|cc}
\hline
                                & Misinterpretation Rate~($\downarrow$) & Human Preference~($\uparrow$) \\ \hline
SD           & 63.0          & 9.4                            \\ \hline
SD-HRV~(Ours)     & \textbf{15.9} & \textbf{80.9}                   \\ \hline
Cannot Determine~/~Both Equally & -             & 9.7                                 \\ \hline
\end{tabular}}
\label{tab:appendix_misinterpretation_human_evaluation}
\end{table}
