# Supplementary material for: Cross-Attention Head Position Patterns Can Align with Human Visual Concepts in Text-to-Image Generative Models
Source: arXiv:2412.02237 source file (2025-02-24)
Supplement: Supplementary file 4 [file Appendix_visual_concepts.tex]

\begin{table}[ht]
\caption{34 visual concepts in the concept-word mapping set. Words corresponding to each concept are listed in our core codebase.}
\centering
\begin{tabular}{ll}
\hline
\textbf{Visual concept} &  \\ \hline
\begin{tabular}[c]{@{}l@{}}Color, Animals, Plants, Fruits and   Vegetables, People, Vehicles, Buildings, \\ Furniture, Electronics, Clothing,   Accessories, Tools, Toys, Food and Beverages, \\ Books and Documents, Sports   Equipment, Musical Instruments, Written Characters, Shape, \\ Texture, Size, Counting,   Image Style, Material, Lighting Conditions, Facial Expressions, \\ Facial   Features, Poses and Gestures, Nature Scenes, Weather Conditions, \\ Time of Day,   Geo-locations, Brand Logos, Geometric Patterns\end{tabular} & \\
\hline
\end{tabular}
\label{tab:appendix_visual_concepts}
\end{table}
