# Supplementary material for: Cross-Attention Head Position Patterns Can Align with Human Visual Concepts in Text-to-Image Generative Models
Source: arXiv:2412.02237 source file (2025-02-24)
Supplement: Supplementary file 5 [file Appendix_visual_concepts_and_words_tableware.tex]

\begin{table}[h]
\caption{Our concept-word set of concept tableware and 10 corresponding words. }
\centering
\resizebox{\textwidth}{!}{%
\begin{tabular}{@{}ll@{}}
\toprule
\textbf{Visual Concept} &  \textbf{Words} \\ \toprule
Tableware & dinner plate, soup bowl, teapot, coffee cup, mug, wine glass, cutlery, sauce boat, butter dish, saucer
\\ 
\bottomrule
\end{tabular}%
}
\label{tab:appendix_visual_concepts_and_words}
\end{table}
